# Supplementary material for: Learning Uncertainty For Safety-Oriented Semantic Segmentation In Autonomous Driving
Source: arXiv:2105.13688 source file (2021-05-28)
Supplement: Supplementary file 1 [file supp.tex]

\appendix
\addcontentsline{toc}{section}{Appendices}
\section*{APPENDIX}

\section{Additional qualitative results}
In \autoref{fig:full_uncertainty_map} we show results on every noise. We test: rain (\ie grey line on the image) and patches (\ie rectangles of uniform color and random sizes). We can see that, just as glare, \obsnet is able to detect both aleatoric and epistemic uncertainty. Distillation fail to detect such uncertainty as is train to predict the same output as the one of the teacher. 

Such behaviour can be see on \autoref{fig:full_safety_map}. Here, we fix a precision threshold of 95\%, we rank each pixels of the image by uncertainty, then we try to make the most prediction without falling under the threshold. We can see that \obsnet is able to make good prediction in nearly all images, where \mcdropout and distillation can not.

\begin{figure}[h]
    \centering
    \includegraphics[width=\linewidth]{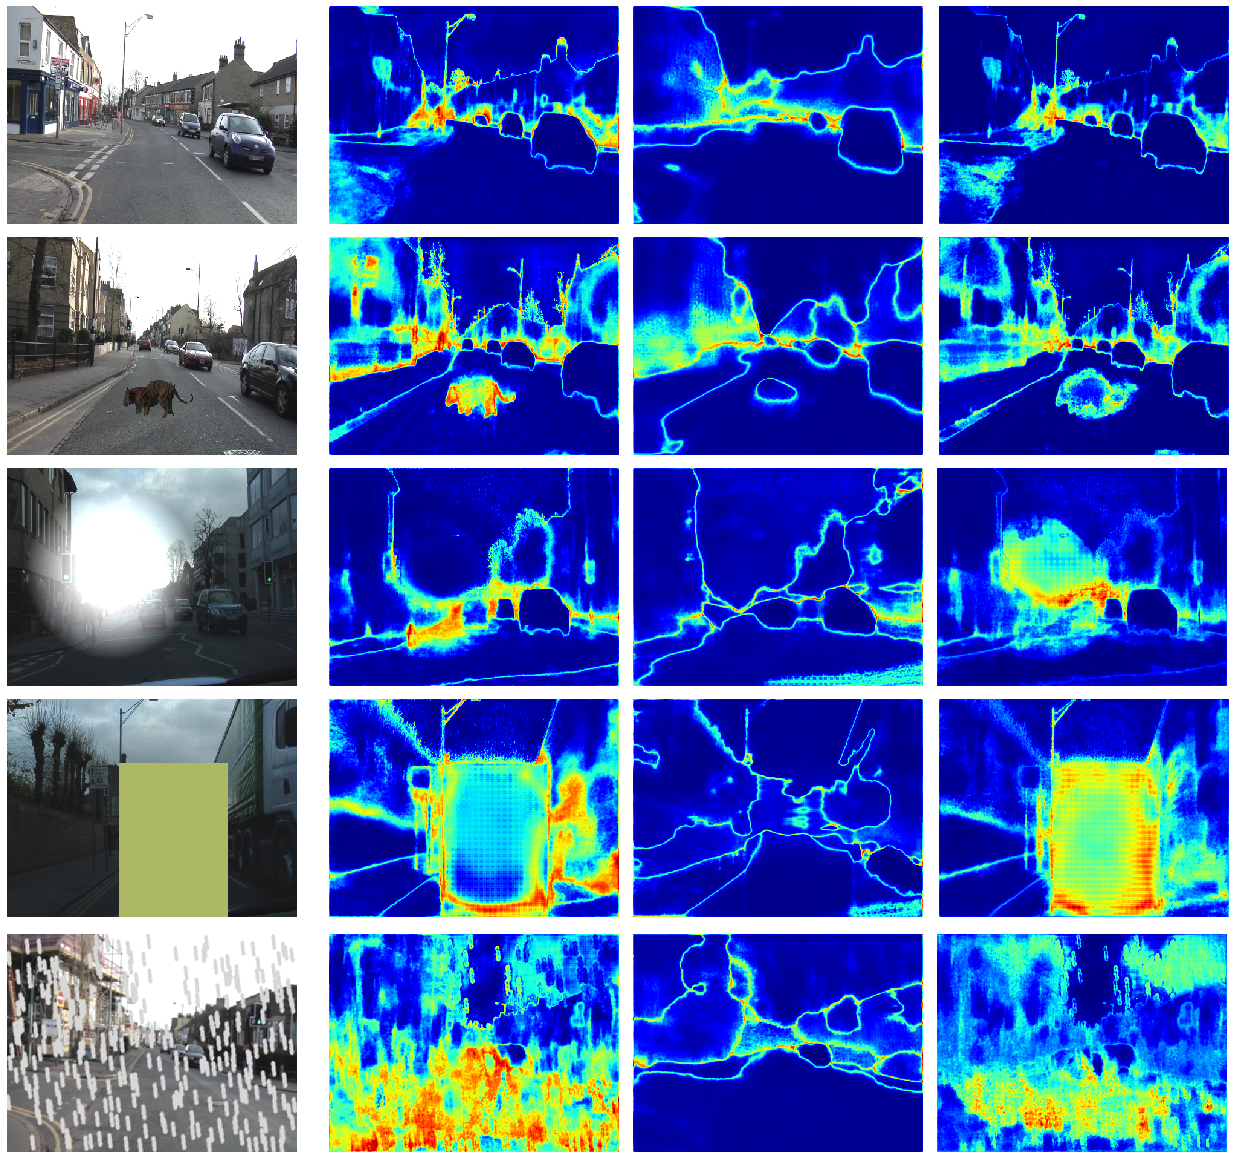}
    \caption{Uncertainty map. From column left to right: Input image, \mcdropout uncertainty, distillation uncertainty, and \obsnet uncertainty. We add two noises which are rain and patch.}
    \label{fig:full_uncertainty_map}
\end{figure}

\begin{figure}[h]
    \centering
    \includegraphics[width=\linewidth]{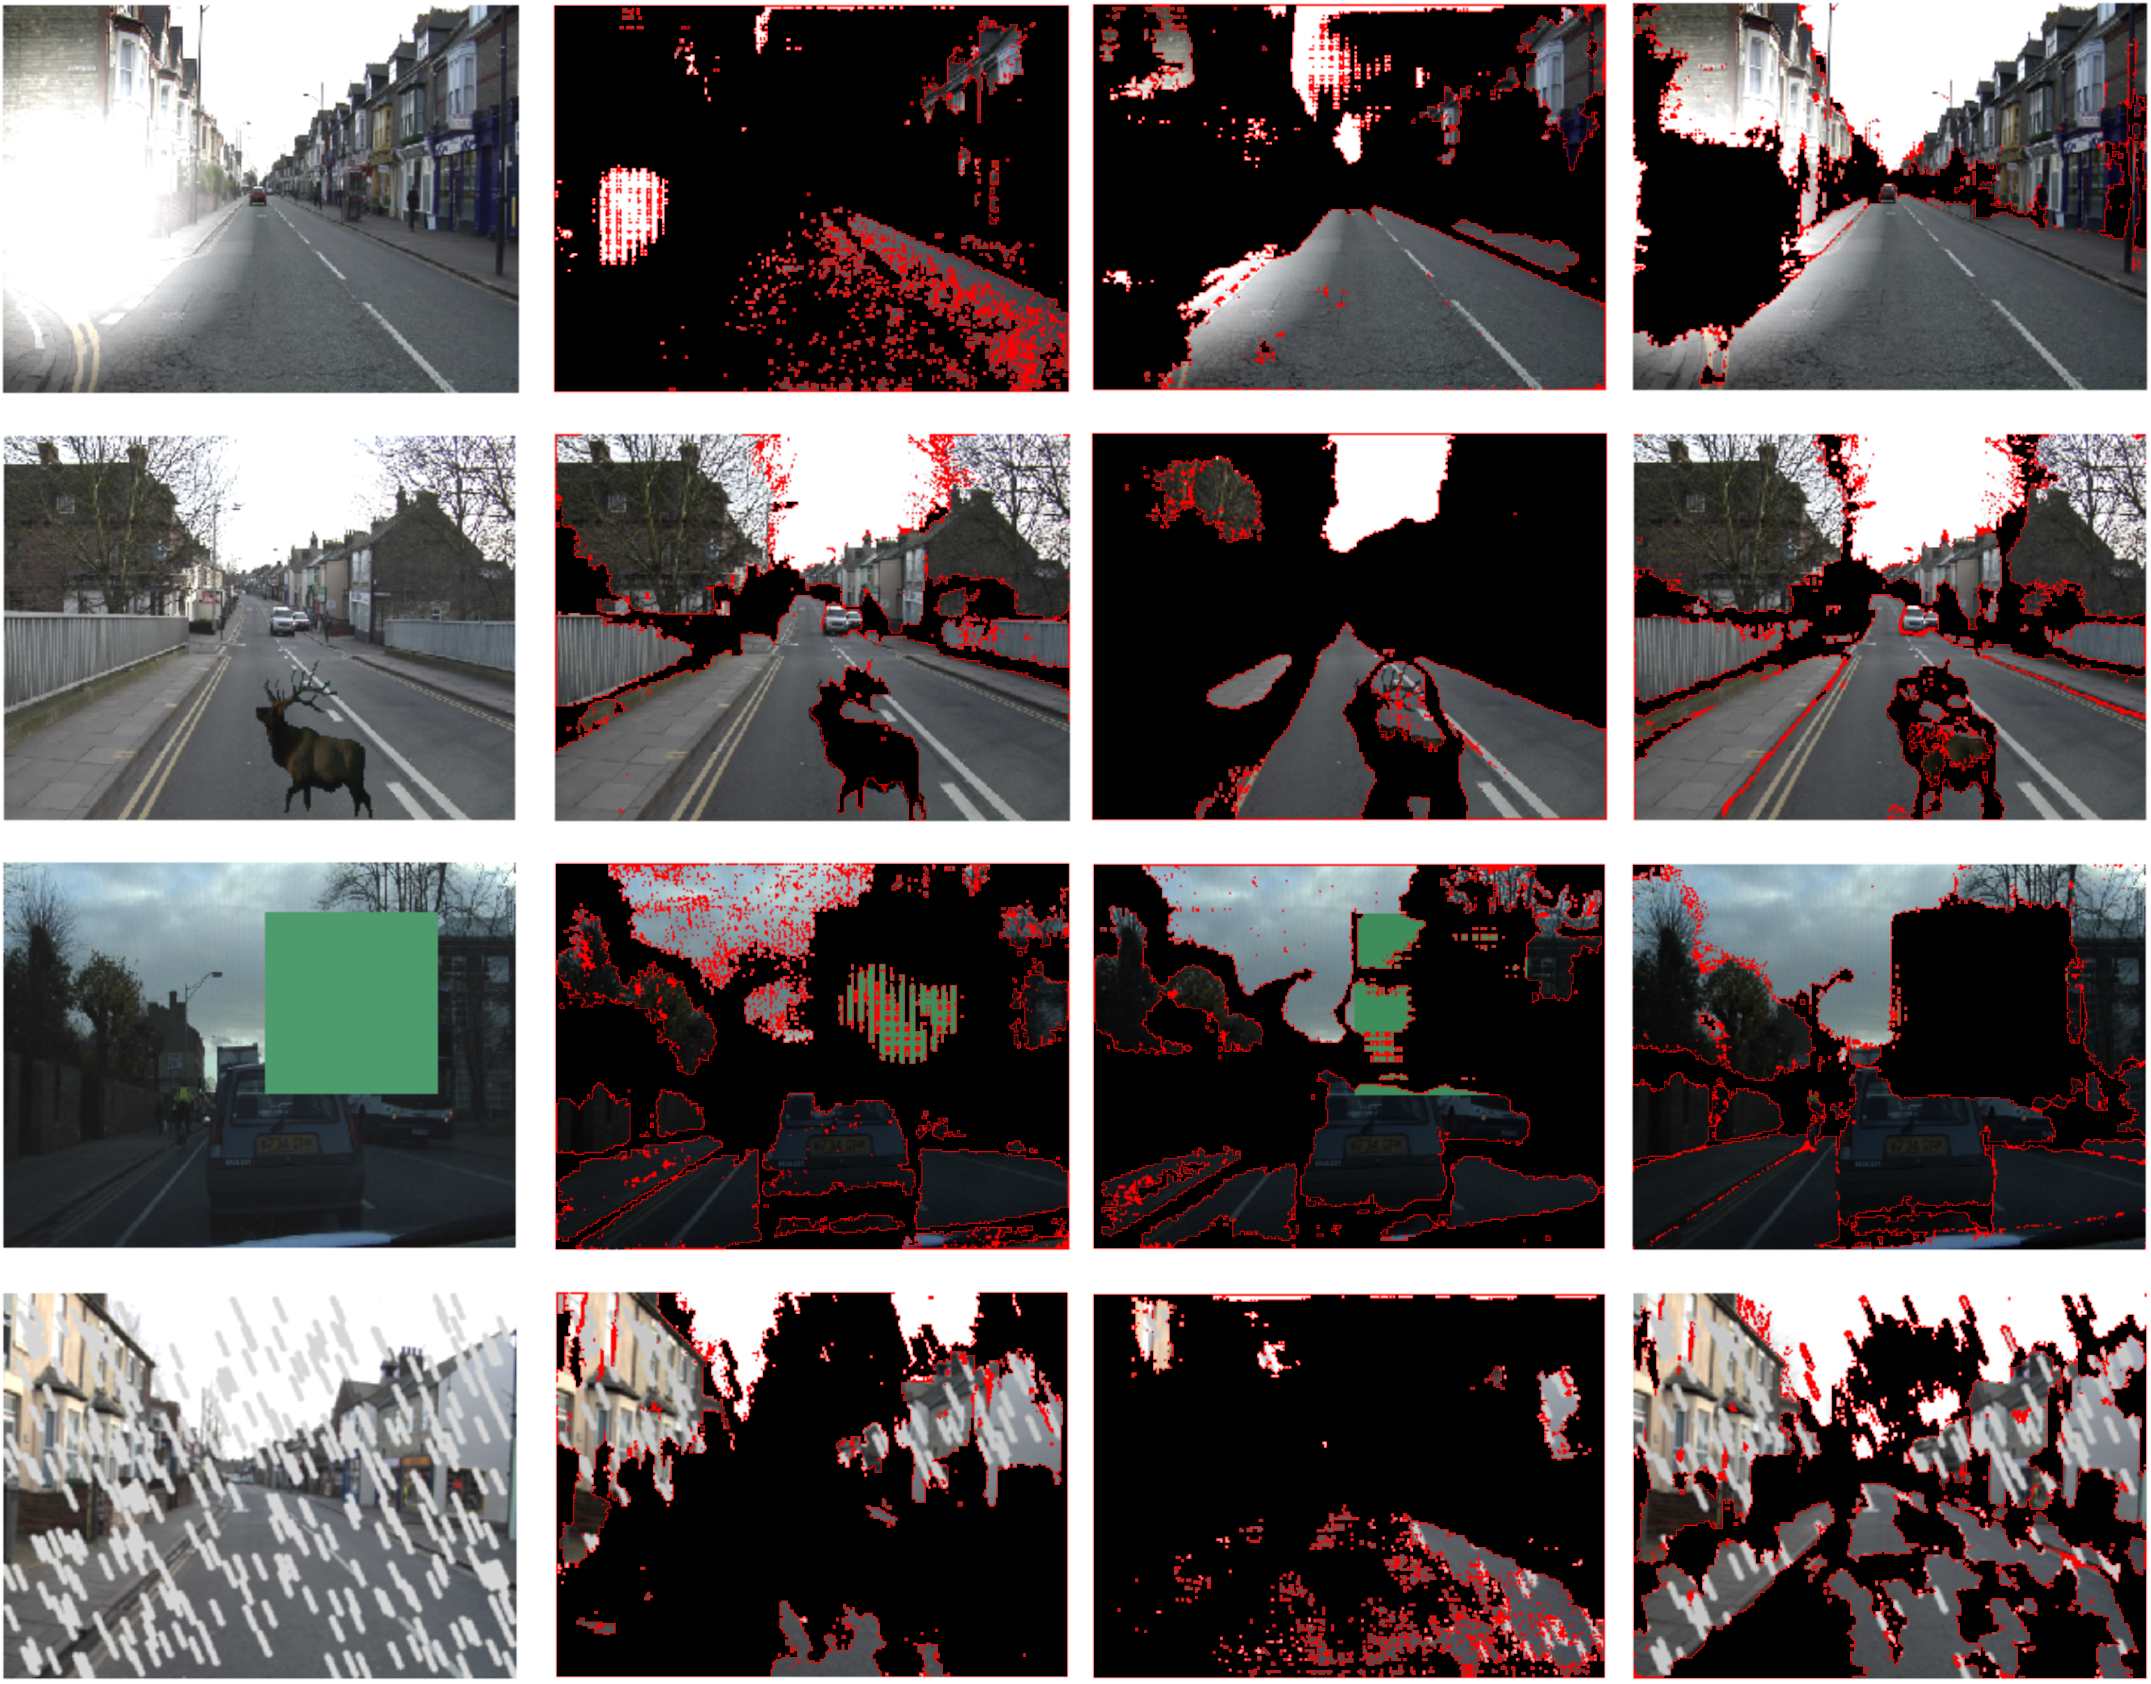}
    \caption{Coverage of the safe predictions. In black and red, where the uncertainty leads the overall precision to fall under 95\%. From left to right: original image, \mcdropout, distillation, and \obsnet.}
    \label{fig:full_safety_map}
\end{figure}

\section{Aleatoric additional results}
In \autoref{tab:aleatoric_table_glare}, \autoref{tab:aleatoric_table_rain} and \autoref{tab:aleatoric_table_square}, we show the complete results for aleatoric uncertainty. We can see that even if \obsnet is train on an other noise, it is able to achieve good result. Moreover, train ObsNet with several noises signiﬁcantly improves the performances for all noises. We can then use many more noise to be more robust to any kind of situation for autonomous driving (e.g., snow, stain, or every low light).

\begin{table*}
 \centering
  \begin{tabular}{cccccccccccc} \toprule
    Test Glare      & Method                   & Train    & R@P=0.95       & AuPR           & Trigger 75\%   \\  \hline
	no-retrain      & \mcdropout T=50          & -        &  0.1 $\pm$ 0.1 & 83.9 $\pm$ 0.1 & 18.9 $\pm$ 1.5 \\
	                & \mcdropout T=2           & -        &  0.0 $\pm$ 0.0 & 83.7 $\pm$ 0.2 & 15.5 $\pm$ 1.6 \\ 
	                & Softmax                  & -        &  1.0 $\pm$ 0.3 & 90.5 $\pm$ 0.8 & 17.2 $\pm$ 2.7 \\ 
	                & Void Class               & -        &  0.3 $\pm$ 0.1 & 82.7 $\pm$ 0.1 &  8.2 $\pm$ 0.9 \\
	                & MCDA T=50                & -        & 44.7 $\pm$ 0.5 & 91.7 $\pm$ 0.2 & 14.3 $\pm$ 2.0 \\ \hline
	                
	Distillation    & w/ T supervised          & patch    &  0.3 $\pm$ 0.1 & 85.7 $\pm$ 0.5 &  4.1 $\pm$ 0.1 \\ 
                    & w/ T unsupervised        & patch    &  1.9 $\pm$ 0.5 & 85.5 $\pm$ 0.7 &  4.3 $\pm$ 0.9 \\ 
	                & w/ T supervised          & rain     &  0.5 $\pm$ 0.0 & 77.1 $\pm$ 0.9 &  3.8 $\pm$ 0.8 \\ 
                    & w/ T unsupervised        & rain     &  0.5 $\pm$ 0.1 & 85.0 $\pm$ 0.5 &  4.2 $\pm$ 0.8 \\ 
                    & w/ T supervised          & glare    &  0.0 $\pm$ 0.3 & 83.3 $\pm$ 0.2 &  2.2 $\pm$ 0.8 \\ 
		            & w/ T unsupervised        & glare    &  1.6 $\pm$ 0.1 & 84.1 $\pm$ 0.3 &  3.0 $\pm$ 0.9 \\
		            & w/ T supervised          & all      &  0.0 $\pm$ 0.0 & 81.9 $\pm$ 0.3 &  1.7 $\pm$ 0.8 \\ 
                    & w/ T unsupervised        & all      &  1.1 $\pm$ 0.3 & 85.9 $\pm$ 0.2 &  3.1 $\pm$ 1.7 \\  \hline
                    
	\obsnet (OURS)  & from \mcdropout          & patch    & 46.7 $\pm$ 1.3 & 92.3 $\pm$ 0.3 & 15.1 $\pm$ 2.1 \\
                    %& from GT                  & patch    & 54.5 $\pm$ 1.1 & 93.8 $\pm$ 0.3 & 26.2 $\pm$ 1.4 \\ 
                    & from \mcdropout          & rain     & 33.9 $\pm$ 1.1 & 90.8 $\pm$ 0.3 & 18.3 $\pm$ 1.0 \\
                    %& from GT                  & rain     & 39.5 $\pm$ 0.3 & 91.9 $\pm$ 0.2 & 20.3 $\pm$ 1.1 \\
                    & from \mcdropout          & glare    & 68.4 $\pm$ 0.9 & 95.3 $\pm$ 0.1 & 23.2 $\pm$ 1.5 \\ 
	                %& from GT                  & glare    & 79.4 $\pm$ 0.5 & 96.6 $\pm$ 0.1 & 39.2 $\pm$ 2.8 \\
	                & from \mcdropout          & all      & \textbf{76.1 $\pm$ 0.5} & \textbf{96.1 $\pm$ 0.1} & \textbf{33.5 $\pm$ 1.8} \\
                    %& from GT                  & all      & 79.3 $\pm$ 0.8 & 96.6 $\pm$ 0.1 & 37.9 $\pm$ 1.4 \\
                    \bottomrule
  \end{tabular}
  \caption{Evaluation of aleatoric uncertainty, tested on glare.}
  \label{tab:aleatoric_table_glare}
\end{table*}

\begin{table*}
 \centering
  \begin{tabular}{cccccccccccc} \toprule
    Test Rain       & Method                   & Train    & R@P=0.95       & AuPR           & Trigger 33\%  \\  \hline
	no-retrain      & \mcdropout T=50          & -        & 10.3 $\pm$ 0.8 & 74.9 $\pm$ 0.5 & 5.6 $\pm$ 0.6 \\
	                & \mcdropout T=2           & -        &  7.3 $\pm$ 0.7 & 73.3 $\pm$ 0.5 & 1.5 $\pm$ 0.3 \\ 
	                & Softmax                  & -        &  6.1 $\pm$ 2.0 & 72.6 $\pm$ 0.3 & 1.2 $\pm$ 0.3 \\ 
	                & Void Class               & -        &  7.2 $\pm$ 3.5 & 73.0 $\pm$ 0.1 & 1.3 $\pm$ 0.3 \\
	                & MCDA T=50                & -        &  6.2 $\pm$ 0.4 & 69.6 $\pm$ 0.3 & 0.2 $\pm$ 0.2 \\ \hline
	                
	Distillation    & w/ T supervised          & glare    &   0.0 $\pm$ 0.0 & 55.0 $\pm$ 0.6 &  0.0 $\pm$ 0.0 \\ 
		            & w/ T unsupervised        & glare    &   0.1 $\pm$ 0.1 & 54.1 $\pm$ 0.7 &  0.0 $\pm$ 0.0 \\  
	                & w/ T supervised          & patch    &  0.0 $\pm$ 0.0 & 54.1 $\pm$ 0.4 &  0.0 $\pm$ 0.0 \\ 
                    & w/ T unsupervised        & patch    &  0.0 $\pm$ 0.0 & 53.4 $\pm$ 0.5 &  0.0 $\pm$ 0.0\\  
	                & w/ T supervised          & rain     &  0.0 $\pm$ 0.0 & 47.6 $\pm$ 0.8 &  0.0 $\pm$ 0.0 \\  
                    & w/ T unsupervised        & rain     &  0.0 $\pm$ 0.0 & 51.1 $\pm$ 0.2 &  0.0 $\pm$ 0.0 \\
                    & w/ T supervised          & all      &  0.0 $\pm$ 0.0 & 53.7 $\pm$ 0.4 &  0.0 $\pm$ 0.0\\ 
                    & w/ T unsupervised        & all      &  0.0 $\pm$ 0.0 & 61.1 $\pm$ 0.2 &  0.0 $\pm$ 0.0\\\hline
                    
	\obsnet (OURS)  & from \mcdropout          & glare    &  3.1 $\pm$ 0.5 & 69.3 $\pm$ 0.6 &  0.3 $\pm$ 0.4 \\
	                %& from GT                  & glare    & 12.6 $\pm$ 1.0 & 75.5 $\pm$ 0.3 &  4.0 $\pm$ 0.1 \\ 
	                & from \mcdropout          & patch    &  3.1 $\pm$ 0.6 & 70.4 $\pm$ 0.6 &  0.8 $\pm$ 0.4 \\
                    %& from GT                  & patch    &  9.7 $\pm$ 0.9 & 75.3 $\pm$ 0.5 &  4.2 $\pm$ 1.4 \\ 
	                & from \mcdropout          & rain     & 32.5 $\pm$ 0.8 & 86.9 $\pm$ 0.2 & 24.7 $\pm$ 1.2 \\
                    %& from GT                  & rain     & 36.7 $\pm$ 0.8 & 88.9 $\pm$ 0.1 & 32.5 $\pm$ 2.7 \\
                    & from \mcdropout          & all      & \textbf{33.2 $\pm$ 1.3} & \textbf{87.2 $\pm$ 0.2} & \textbf{25.1 $\pm$ 2.0}\\
                    %& from GT                  & all      & 43.4 $\pm$ 1.1 & 90.1 $\pm$ 0.2 & 34.7 $\pm$ 0.9 \\
\bottomrule
  \end{tabular}
  \caption{Evaluation of aleatoric uncertainty, tested on rain.}
  \label{tab:aleatoric_table_rain}
\end{table*}

\begin{table*}
 \centering
  \begin{tabular}{cccccccccccc} \toprule
    Test Patch      & Method                   & Train    & R@P=0.95       & AuPR           & Trigger 75\%   \\  \hline
	no-retrain      & \mcdropout T=50          & -        & 63.9 $\pm$ 7.3 & 94.9 $\pm$ 0.7 & 19.6 $\pm$ 2.9 \\
	                & \mcdropout T=2           & -        & 23.4 $\pm$ 5.1 & 93.5 $\pm$ 0.5 & 18.5 $\pm$ 2.5 \\ 
	                & Softmax                  & -        &  0.3 $\pm$ 0.1 & 90.3 $\pm$ 0.3 & 15.9 $\pm$ 1.2 \\ 
	                & Void Class               & -        &  0.2 $\pm$ 0.1 & 86.4 $\pm$ 0.3 &  8.7 $\pm$ 1.1 \\
	                & MCDA T=50                & -        & 32.0 $\pm$ 1.3 & 90.4 $\pm$ 0.2 & 12.4 $\pm$ 1.1 \\ \hline
	                
	Distillation    & w/ T supervised          & glare    &   0.0 $\pm$ 0.0 & 85.2 $\pm$ 0.3 &  3.1 $\pm$ 0.4 \\ 
		            & w/ T unsupervised        & glare    &   1.3 $\pm$ 0.2 & 84.8 $\pm$ 0.6 &  3.2 $\pm$ 0.9 \\
                    & w/ T supervised          & rain     &   0.0 $\pm$ 0.0 & 54.0 $\pm$ 0.1 & 0.0 $\pm$ 0.0 \\ 
                    & w/ T unsupervised        & rain     &   0.0 $\pm$ 0.0 & 54.1 $\pm$ 0.4 & 0.0 $\pm$ 0.0 \\  
		            & w/ T supervised          & patch    &   1.4 $\pm$ 0.4 & 79.6 $\pm$ 0.7 &  4.4 $\pm$ 0.9 \\
                    & w/ T unsupervised        & patch    &   2.2 $\pm$ 0.3 & 82.7 $\pm$ 0.5 &  4.5 $\pm$ 1.5 \\ 
                    & w/ T supervised          & all      &   0.0 $\pm$ 0.0 & 79.5 $\pm$ 0.7 &  1.9 $\pm$ 0.9 \\
                    & w/ T unsupervised        & all      &   1.3 $\pm$ 0.3 & 84.7 $\pm$ 0.6 &  3.4 $\pm$ 1.3 \\  \hline

	\obsnet (OURS)  & from \mcdropout          & glare    &  46.5 $\pm$ 0.9 & 92.6 $\pm$ 0.2 & 15.2 $\pm$ 2.1 \\
	                %& from GT                  & glare    &  53.6 $\pm$ 0.7 & 93.6 $\pm$ 0.1 & 23.2 $\pm$ 0.8 \\  
	                & from \mcdropout          & rain     &   2.7 $\pm$ 0.5 & 70.2 $\pm$ 0.2 & 0.9 $\pm$ 0.6 \\
                    %& from GT                  & rain     &  10.5 $\pm$ 0.5 & 75.2 $\pm$ 0.3 & 3.5 $\pm$ 0.8 \\
	                & from \mcdropout          & patch    &  72.5 $\pm$ 0.4 & 95.6 $\pm$ 0.1 & 23.6 $\pm$ 2.7 \\ 
                    %& from GT                  & patch    &  82.3 $\pm$ 0.4 & 96.9 $\pm$ 0.9 & 36.7 $\pm$ 1.7 \\
                    & from \mcdropout          & all      & \textbf{77.5 $\pm$ 0.4} & \textbf{96.1 $\pm$ 0.1} & \textbf{30.5 $\pm$ 1.4} \\
                    %& from GT                  & all      & 81.4 $\pm$ 0.3 & 96.8 $\pm$ 0.0 & 35.2 $\pm$ 2.2 \\
\bottomrule
  \end{tabular}
  \caption{Evaluation of aleatoric uncertainty, tested on patch.}
  \label{tab:aleatoric_table_square}
\end{table*}

Furthermore, we show in \autoref{fig:pr_curve_supp} the Precision-recall curves for every noises. Our work (in green), outperform every other methods for aleatoric uncertainty. 
\begin{figure}
\centering
\begin{subfigure}{.25\textwidth}
  \centering
  \includegraphics[width=\linewidth]{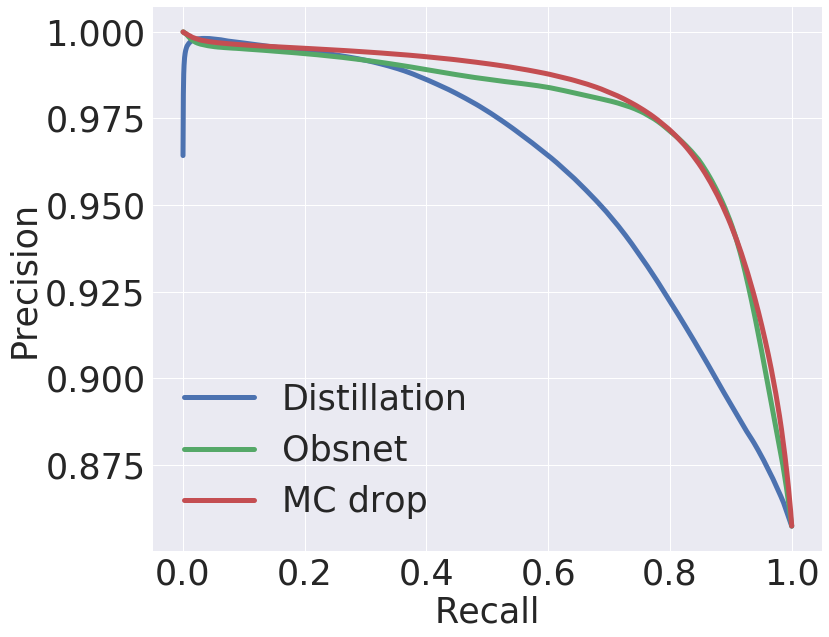}
  \caption{Normal.}\label{fig:pr_curve_no_noise}
\end{subfigure}
\begin{subfigure}{.23\textwidth}
  \centering
  \includegraphics[width=\linewidth]{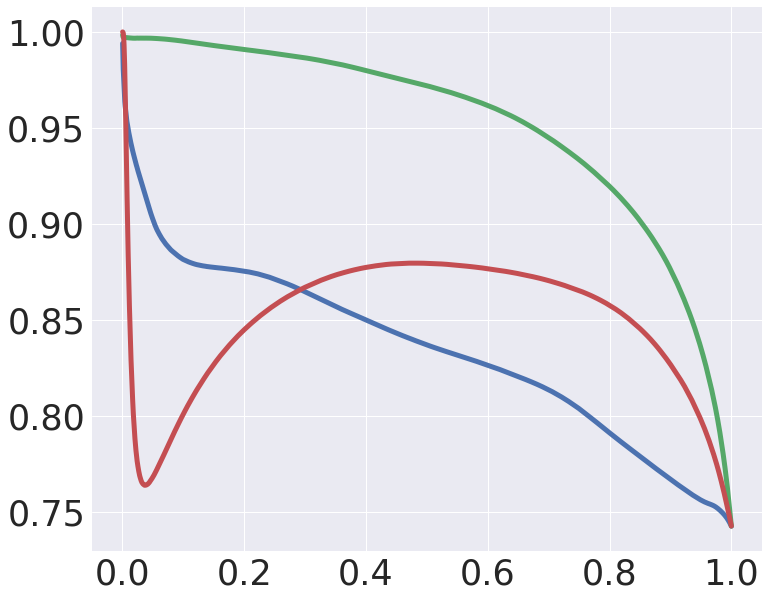}
  \caption{Glare.}\label{fig:pr_curve_no_noise}
\end{subfigure}
\begin{subfigure}{.23\textwidth}
  \centering
  \includegraphics[width=\linewidth]{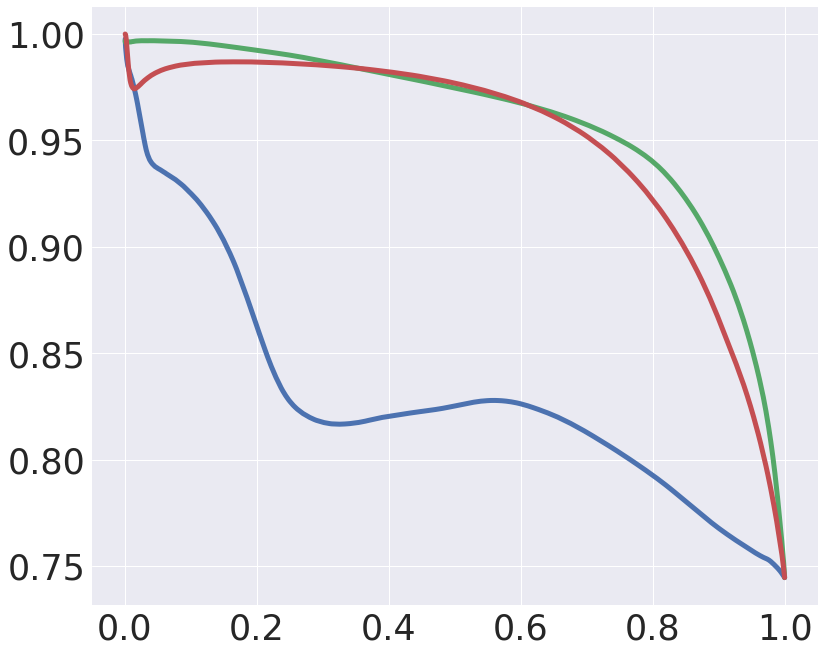}
  \caption{Square.}\label{fig:pr_curve_animals}
\end{subfigure}
\begin{subfigure}{.23\textwidth}
  \centering
  \includegraphics[width=\linewidth]{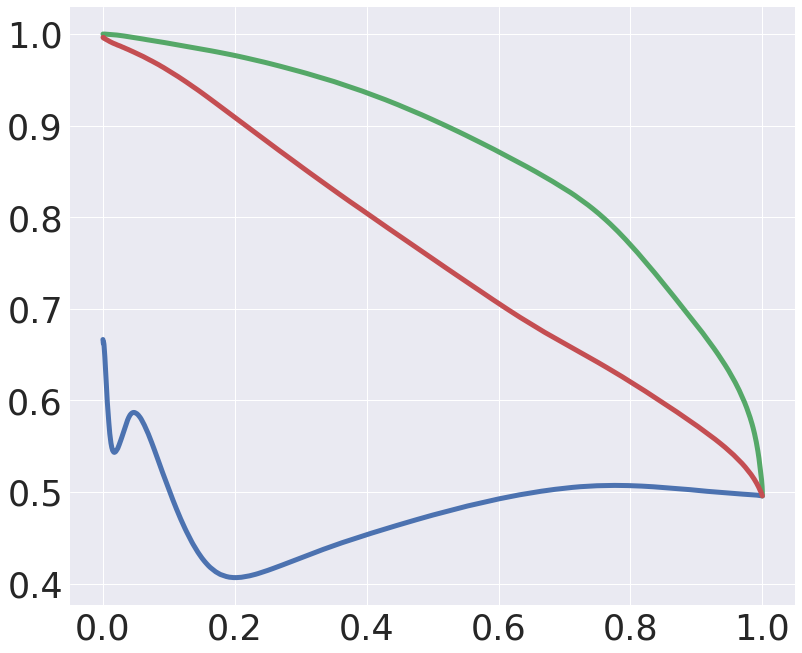}
  \caption{Rain.}\label{fig:pr_curve_glare}
\end{subfigure}
\caption{Precision-Recall Curves for aleatoric uncertainty. We compare the cases where we added: \textbf{(a)} No noise, \textbf{(b)} random glare effect, \textbf{(c)} random patch and \textbf{(d)} rain effect}
\label{fig:pr_curve_supp}
\end{figure}

\section{Uncertainty Label c}
We show in \autoref{fig:fig_label_epis} the self-supervised label c from epistemic uncertainty. The red pixels on the most right images are the pixels where the uncertainty are above the safety parameters $\delta$. It shows where we learn to maximize the the KL divergence (red pixel) and where we learn to minimize it (in blue). 

For aleatoric uncertainty estimation \autoref{fig:fig_label_alea}, we see in red the pixels where the noise shifts the output distribution above the safety parameter $\delta$. Thus, leading to aleatoric uncertainty (red pixels) or not (blue pixels). We can see that even if some pixels are overlap by a the glare, the corresponding label is $c = + 1$. This mean that if the target network can predict the right class for this pixel, then there is enough information in the data to make a safe prediction.   

\begin{figure}
\hspace{10pt}
\centering
\begin{subfigure}{.3\textwidth}
  \centering
  \includegraphics[width=\linewidth]{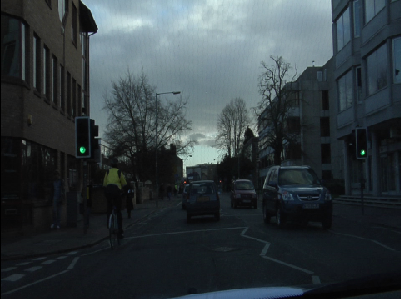}
  \caption{Input.}
  \label{fig:method1}
\end{subfigure}%
\hspace{0.4cm}
\begin{subfigure}{.3\textwidth}
  \centering
  \includegraphics[width=\linewidth]{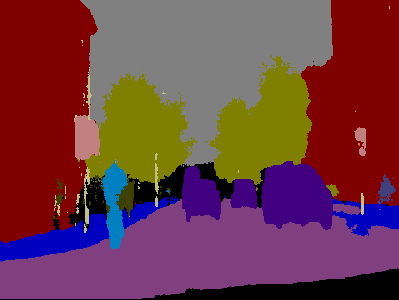}
  \caption{Prediction.}
  \label{fig:method2}
\end{subfigure}%
\hspace{0.4cm}
\begin{subfigure}{.3\textwidth}
  \centering
  \includegraphics[width=\linewidth]{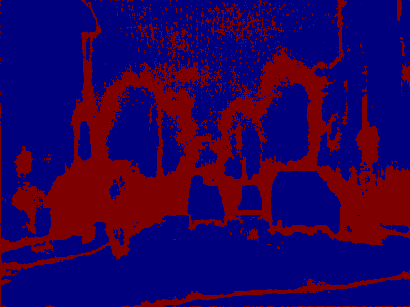}
  \caption{Uncertainty labels $c$}
  \label{fig:method3}
\end{subfigure}
\caption{Epistemic uncertainty labels to train \obsnet. The last image shows self-supervised labels, $c=+1$ in blue and $c=-1$ in red.}
\label{fig:fig_label_epis}
\end{figure}

\begin{figure}
\hspace{10pt}
\centering
\begin{subfigure}{.3\textwidth}
  \centering
  \includegraphics[width=\linewidth]{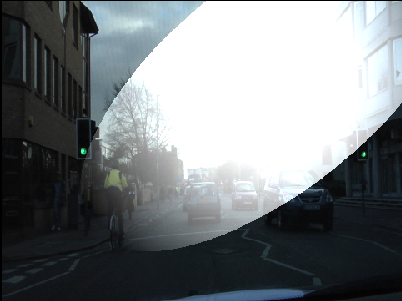}
  \caption{Image with noise.}
  \label{fig:method4}
\end{subfigure}%
\hspace{0.4cm}
\begin{subfigure}{.3\textwidth}
  \centering
  \includegraphics[width=\linewidth]{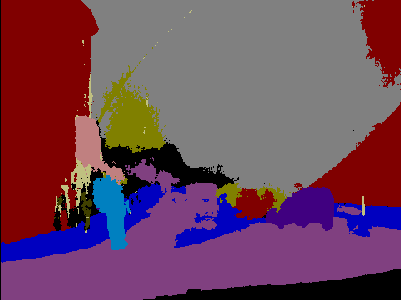}
  \caption{Prediction with noise.}
  \label{fig:method5}
\end{subfigure}%
\hspace{0.38cm}
\begin{subfigure}{.3\textwidth}
  \centering
  \includegraphics[width=\linewidth]{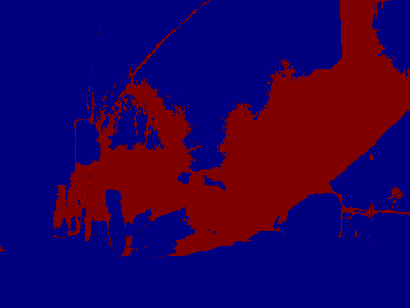}
  \caption{Uncertainty labels $c$}
  \label{fig:method6}
\end{subfigure}
\hspace{13pt}%
\caption{Aleatoric uncertainty labels to train \obsnet. The last image shows self-supervised labels, $c=+1$ in blue and $c=-1$ in red.}
\label{fig:fig_label_alea}
\end{figure}

\section{\obsnet Architecture}
For \obsnet model, we replicate Bayesian SegNet architecture, see \autoref{tab:architec}. A \emph{ConvBlock} is compose of Convolution layer, Batch Normalization and ReLU activation. Before training \obsnet, we copied the weight from the target network. For residual connection, we use the activation of the target network from the same position. 
For training, we use SGD with momentum and weight decay of $5e-4$, we use a learning rate of $1e-3$, batch size equal to 5 and 50 epoch. Moreover, we reduce the learning rate by 2 after 20 and 40 epochs. We select the best \obsnet on the validation set of CamVid.

\begin{table}[h!]
\caption{ObsNet Architecture.}
\centering
\scalebox{0.8}{%
\begin{tabular}{@{}ccc@{}}
\toprule
      &  & ObsNet                         \\ \cmidrule(r){1-3}% \cmidrule(l){3-3} 
      &  & Image intput (3, 480, 360)     \\ \cmidrule(r){1-1} \cmidrule(l){3-3} 
Down1 &  & ConvBlock(3, 64)               \\
      &  & ConvBlock(64, 64) + residual   \\
      &  & MaxPool(2, 2)                      \\ \cmidrule(r){1-1} \cmidrule(l){3-3} 
Down2 &  & ConvBlock(64, 128)             \\
      &  & ConvBlock(128, 128) + residual \\
      &  & MaxPool(2, 2)                      \\ \cmidrule(r){1-1} \cmidrule(l){3-3} 
Down3 &  & ConvBlock(128, 256)            \\
      &  & ConvBlock(256, 256)            \\
      &  & ConvBlock(256, 256) + residual \\
      &  & MaxPool(2, 2)                      \\
      &  & Dropout2D(p=.5)                    \\ \cmidrule(r){1-1} \cmidrule(l){3-3} 
down4 &  & ConvBlock(256, 512)            \\
      &  & ConvBlock(512, 512)            \\
      &  & ConvBlock(512, 512) + residual \\
      &  & MaxPool(2, 2)                  \\
      &  & Dropout2D(p=.5)                    \\ \cmidrule(r){1-1} \cmidrule(l){3-3} 
down5 &  & ConvBlock(512, 512)            \\
      &  & ConvBlock(512, 512)            \\
      &  & ConvBlock(512, 512) + residual \\
      &  & MaxPool(2, 2)                  \\
      &  & Dropout2D(p=.5)                    \\ \cmidrule(r){1-1} \cmidrule(l){3-3} 
up5   &  & UpSampling(2, 2)               \\
      &  & ConvBlock(512, 512)            \\
      &  & ConvBlock(512, 512)            \\
      &  & ConvBlock(512, 512) + residual \\
      &  & Dropout2D(p=.5)                    \\ \cmidrule(r){1-1} \cmidrule(l){3-3} 
up4   &  & UpSampling(2, 2)               \\
      &  & ConvBlock(512, 512)            \\
      &  & ConvBlock(512, 512)            \\
      &  & ConvBlock(512, 256) + residual \\
      &  & Dropout2D(p=.5)                    \\ \cmidrule(r){1-1} \cmidrule(l){3-3} 
up3   &  & UpSampling(2, 2)               \\
      &  & ConvBlock(256, 256)            \\
      &  & ConvBlock(256, 256)            \\
      &  & ConvBlock(256, 128) + residual \\
      &  & Dropout2D(p=.5)                    \\ \cmidrule(r){1-1} \cmidrule(l){3-3} 
up2   &  & UpSampling(2, 2)               \\
      &  & ConvBlock(128, 128)            \\
      &  & ConvBlock(128, 64) + residual  \\ \cmidrule(r){1-1} \cmidrule(l){3-3} 
up1   &  & UpSampling(2, 2)               \\
      &  & ConvBlock(64, 64)              \\
      &  & ConvBlock(64, 12) + residual   \\ \cmidrule(r){1-1} \cmidrule(l){3-3} 
      &  & FullyConnected(12, 12)         \\
      &  & Softmax                        \\ \bottomrule
\end{tabular}}
\label{tab:architec}
\end{table}

\section{Patches Color Space}
We use different colors for training and testing on patches. We use blue, magenta, white and turquoise to train: \autoref{fig:color_train}, and black, red, green and yellow to test: \autoref{fig:color_test}.
\begin{figure}[h!]
\centering
\begin{subfigure}{.3\textwidth}
  \centering
  \includegraphics[width=\linewidth]{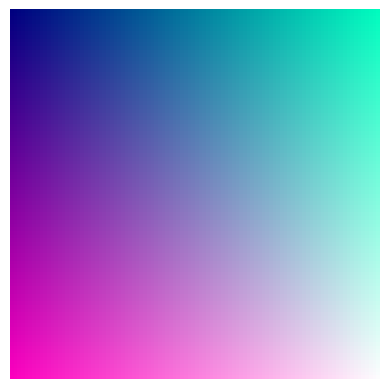}
  \caption{Train.}\label{fig:color_train}
\end{subfigure}
\begin{subfigure}{.3\textwidth}
  \centering
  \includegraphics[width=\linewidth]{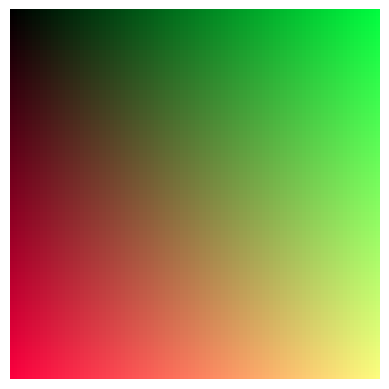}
  \caption{Test.}\label{fig:color_test}
\end{subfigure}
\caption{Patches Color Space.}
\label{fig:color}
\end{figure}
